# Supplementary material for: Accelerated Molecular Dynamics through stochastic iterations to strengthen yield of path hopping over upper states (SISYPHUS)
Source: arXiv:1212.6649 ancillary file (2013-01-02)
Supplement: Supplementary file 1 [file supplementary_materials.pdf]

# Accelerated Molecular Dynamics simulations through SISYPHUS: Supplemental Materials

Pratyush Tiwary and Axel van de Walle
*School of Engineering, Brown University, Providence, Rhode Island 02912, USA*
(Dated: December 27, 2012)

## I. NON-UNIFORM GRID FOR ADIABATIC SWITCHING: A RIGOROUS BASIS

This section concerns with the evaluation of the second integral in adiabatic switching (see Eqs. (5-7) in main text, and Eqs. 1-3 below) and rigorously justifies the non-uniform integration grid scheme to evaluate $R$ which can be made finer as $\alpha \to 0$ but kept coarse for larger $\alpha$, leading to significant computational efficiency. In the main text, we talk about the rate $t_{\mathbf{W}}^{-1}$, where

$$
\begin{aligned}
t_{\mathbf{W}}^{-1} &= \lim_{w\to 0} \frac{\int \frac{\bar{v}}{w} 1\left(x \in S_w\right) e^{-\beta \hat{V}(x,0)} dx}{\int e^{-\beta \hat{V}(x,0)} dx} \\
&= \lim_{w\to 0} \frac{\int \frac{\bar{v}}{w} 1\left(x \in S_w\right) e^{-\beta\left(\hat{V}(x,0)-\hat{V}(x,1)\right)} e^{-\beta \hat{V}(x,1)} dx}{\int e^{-\beta \hat{V}(x,1)} dx} \left(\frac{\int e^{-\beta \hat{V}(x,1)} dx}{\int e^{-\beta \hat{V}(x,0)} dx}\right) \\
&\equiv \lim_{w\to 0} \left\langle \frac{\bar{v} 1\left(x \in S_w\right)}{w} e^{-\beta\left(\hat{V}(x,0)-\hat{V}(x,1)\right)} \right\rangle_1 R
\end{aligned} \tag{1}
$$

where $dx$ denotes a differential volume in 3-N dimensional configuration space for N particles, the integration being performed over entire configuration space within the well $\mathbf{W}$ and the expected value $\langle \cdots \rangle_\alpha$ in Eq.(3) is defined by

$$
\langle \cdots \rangle_\alpha = \frac{\int \left(\cdots\right) e^{-\beta \hat{V}(x,\alpha)} dx}{\int e^{-\beta \hat{V}(x,\alpha)} dx} \tag{2}
$$

$R$ can be re-expressed as

$$
\begin{aligned}
R &= \frac{\int e^{-\beta \hat{V}(x,1)} dx}{\int e^{-\beta \hat{V}(x,0)} dx} \\
&= \exp\left(\ln \int e^{-\beta \hat{V}(x,1)} dx - \ln \int e^{-\beta \hat{V}(x,0)} dx\right) \\
&= \exp\left(\int_0^1 \left(\frac{\partial}{\partial \alpha} \ln \int e^{-\beta \hat{V}(x,\alpha)} dx\right) d\alpha\right) \\
&= \exp\left(-\beta \int_0^1 \frac{\int \frac{\partial \hat{V}(x,\alpha)}{\partial \alpha} e^{-\beta \hat{V}(x,\alpha)} dx}{\int e^{-\beta \hat{V}(x,\alpha)} dx} d\alpha\right) \\
&= \exp\left(-\beta \int_0^1 \left\langle \frac{\partial \hat{V}\left(x,\alpha\right)}{\partial \alpha} \right\rangle_\alpha d\alpha\right)
\end{aligned} \tag{3}
$$

We define the average $\langle \frac{\partial \hat{V}(x,\alpha)}{\partial \alpha} \rangle_\alpha = \langle V^*(x) - V(x) \rangle_\alpha$ as $g(\alpha)$. We make and prove a few claims about the derivatives of $g(\alpha)$. These in turn allow us to use an integral step-size that decreases as $\alpha$ increases. Given that the evaluation of Eq. 3 is the most time-consuming aspect of SISYPHUS, this adaptive grid scheme is crucial. Note that the proof applies only for the linear switching scheme as described in the text.

**Claim I.1.** *$\partial g/\partial \alpha$ is always non-positive and $\partial^2 g/\partial \alpha^2$ is always non-negative*

*Proof.* We explicitly evaluate $\frac{\partial g}{\partial \alpha}$ and $\frac{\partial^2 g}{\partial \alpha^2}$,

$$\begin{aligned}
\frac{\partial g}{\partial \alpha} &= \frac{\partial \langle V^* - V \rangle_\alpha}{\partial \alpha} \\
&= \frac{\partial [\frac{\int dr (V^* - V) e^{-\beta V(\alpha)}}{\int dr e^{-\beta V(\alpha)}}]}{\partial \alpha} \\
&= -\beta \frac{\int dr (V^* - V)^2 e^{-\beta V(\alpha)}}{\int dr e^{-\beta V(\alpha)}} + \beta [\frac{\int dr (V^* - V) e^{-\beta V(\alpha)}}{\int dr e^{-\beta V(\alpha)}}]^2 \\
&= -\beta \{ \langle (V^* - V)^2 \rangle_\alpha - (\langle V^* - V \rangle_\alpha)^2 \}.
\end{aligned}$$

which is $\leq 0$. We thus have verified one part of the claim. We differentiate the above once again with respect to $\alpha$, and get

$$\begin{aligned}
\frac{\partial^2 g}{\partial \alpha^2} &= -\beta \frac{\partial \{ \langle (V^* - V)^2 \rangle_\alpha - (\langle V^* - V \rangle_\alpha)^2 \}}{\partial \alpha} \\
&= -\beta V_0^2 \frac{\partial \{ \langle (1 - \chi/\chi_{cut})^{2m} \rangle_\alpha - (\langle (1 - \chi/\chi_{cut})^m \rangle_\alpha)^2 \}}{\partial \alpha} \\
&= -\beta V_0^2 \frac{\partial \langle variance((1 - \chi/\chi_{cut})^m) \rangle_\alpha}{\partial \alpha}.
\end{aligned}$$

As we increase $\alpha$, the variance of $(1 - \chi/\chi_{cut})^m$ decreases because the distribution of $\chi$ shrinks towards values in close neighborhood of $\chi_{cut}$, since we now have applied increasing bias towards low-$\chi$ states. The above is thus $\geq 0$. We have now verified both parts of the claim. □

## II. SIMULATION SYSTEM AND PARAMETER DETAILS

### A. Vacancy diffusion in Ta

We considered 249 Ta atoms (5x5x5 BCC supercell with 1 vacancy) interacting through the Embedded Atom Method (EAM) potential (Ref. 26), under fully periodic boundary conditions in all 3 directions. For the MD part here, we performed NVT simulations using time step of 2x$10^{-15}$ sec and a Langevin thermostat with coupling constant 1x$10^{-11}$ sec$^{-1}$. Parameters $V_0$ and $\chi_{cut}$ for this simulation have already been provided in Fig. 2 in the main text. The decorrelation time in MD $\tau_c$ was 10 ps. Two values for the lid thickness $w$ in Eq.(1) were taken, 0.01 and 0.005 $\mathring{A}$, and a linear extrapolation was performed to find the limit as $w \to 0$. $p$ in Eq. (9) in main text was kept as 8.

### B. Island ripening on Al (001) surface

We considered 588 Al atoms (6 atomic layers) interacting through the Embedded Atom Method (EAM) potential (Ref. 29). 37 more Al atoms were then randomly deposited on the (001) surface leading to an adatom coverage of around 40% and a total of 625 atoms. The system was then quenched to its nearest local minima using a steepest descent algorithm. Fully periodic boundary conditions in all 3 directions were used. However given that the employed interatomic potential is short-range and goes to 0 around 6$\mathring{A}$, the top-layer of atoms does not interact with its image along z-direction.

For the MD part here, we performed NVT simulations at temperature 300K using time step of 2x$10^{-15}$ sec and a Langevin thermostat with coupling constant 1x$10^{-11}$ sec$^{-1}$. $V_0$ was $2eV$ and $\chi_{cut} - \langle \chi \rangle$ (i.e. relative to average $\chi$ as obtained through NVT MD at 300K) was $0.075a_0$ for this simulation. The decorrelation time in MD $\tau_c$ was 10 ps. Two values for the lid thickness $w$ in Eq.(1) were taken, 0.01 and 0.005 $\mathring{A}$, and a linear extrapolation was performed to find the limit as $w \to 0$. $p$ in Eq. (9) in main text was kept as 10.

### C. Back-of-the-envelope guide for estimating a good choice of $V_0$

Although the eventual dynamics from SISYPHUS is not very sensitive to the choice of the parameter $V_0$ (see Fig. 2 in main text for an illustration), an appropriately picked $V_0$ can still lead to computational efficiency. We now provide an estimate of $V_0$ for the Ta problem that facilitates more efficient MC simulations.

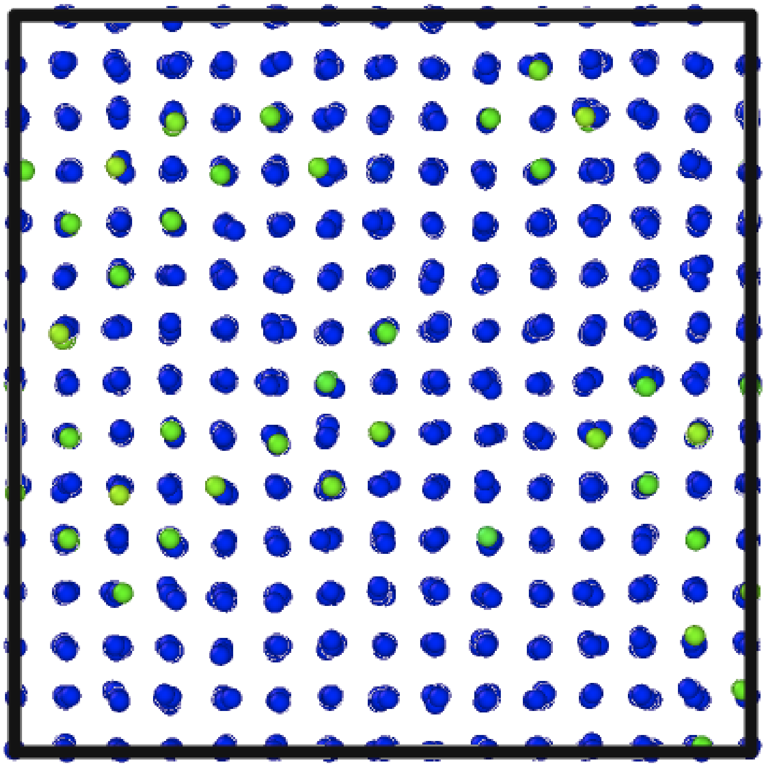

FIG. 1: Superimposed snapshots from a MC$a$ run at 600K for Al (001) island ripening example, viewing along $z$-direction. Green atoms are adatoms, blue atoms are substrate atoms. Each atom visits states well-isolated from other atoms, as can be seen from the intersecting blue (or green) circles.

Let V(x) and $V^*(x)$ denote the true potential and the biased potential respectively. We have Eq. (4) for the biased landscape.

$$V^*(x) = V(x) + V_0(1 - \chi/\chi_{cut})^{0.4}, \chi \leq \chi_{cut}, \tag{4}$$

Let's estimate what range of $V_0$ is needed for the 249 Ta atom system at room temperature, so that the well lid is visited frequently. The acceptance probability for going from a configuration $x_1$ to $x_2$ is given by

$$P = e^{\frac{-V^*(x_2)+V^*(x_1)}{k_BT}} \tag{5}$$

where $V^*(x_1) = V(x_1) + V_0(1 - \chi_1/\chi_{cut})^{0.4}$ and similarly $V^*(x_2)$. $\chi_1$ and $\chi_2$ are the values of the bond distortion function for configurations $x_1$ and $x_2$ respectively.

Now let's look at a scenario where $\chi_1 = \langle\chi\rangle$, and $\chi_2$ corresponds to $x_2 \in S_w$. At room temperature, we find $\langle\chi\rangle \approx 1$ and we choose $\chi_{cut} = 1.6$. $\chi$ here is in units of lattice constant (3.3$\mathring{A}$ for Ta), thus this corresponds to $\chi_{cut} - \langle\chi\rangle \approx 0.2a_0$.

For 90% acceptance probability, $P \approx e^{-0.1}$. This gives

$$\begin{aligned} e^{\frac{-V^*(x_2)+V^*(x_1)}{k_BT}} &\geq e^{-0.1} \text{ , or} \\ e^{\frac{-V(x_2)+V(x_1)+0.5V_0}{k_BT}} &\geq e^{-0.1} \text{ , or} \\ \frac{-V(x_2)+V(x_1)+0.5V_0}{k_BT} &\geq -0.1 \text{ , or} \\ V_0 &\geq \frac{V(x_2)-V(x_1)-0.1k_BT}{0.5} \end{aligned} \tag{6}$$

The standard deviation in potential energy per degree of freedom in the system at room temperature is around $k_B T$, therefore at room temperature the standard deviation in *total potential energy* of the system with 249 atoms is around 0.6eV. We can thus take a typical $V(x_2) - V(x_1) = 0.6eV$. Then at room temperature we get $V_0 \gtrapprox 1.2eV$. This is roughly in the range of values we used in this work - see Figure 2(c) in main text.

## III. A LOOK INTO MC$a$ PART OF THE SIMULATION

One concern that could be raised is if the system happens to escape from one well to another during the decorrelation MC (MC$a$). For the range of $\chi_{cut}$ values considered in this letter, even for the aggressively high ones, we found that the system always stayed inside the well it started in, during the course of any one MC$a$ simulation. We also found that there was no dependence of any of our results on the length of this MC$a$ simulation, as long as it was longer than a few MC passes. In Fig. 1 we corroborate the observation that system stays within well-connected states during MC$a$ by providing a superposition of the snapshots of states visited during one MC$a$ run, for the case of Al adatom ripening at 300K. As can be seen, each atom visits states well-isolated from other atoms.
